# Supplementary material for: DeLag: Using Multi-Objective Optimization to Enhance the Detection of Latency Degradation Patterns in Service-based Systems
Source: arXiv:2110.11155 source file (2023-04-07)
Supplement: Supplementary file 1 [file appendix.tex]

\appendix
\figref{fig:rq2_box_others} depicts the distributions of the mean F1-score ($Q_{F1}$) for K-means, HC and DeCaf under the different experimental setups defined in \secref{sec:rq2}.
The x-axis labels report the expected distance between the average latency of requests in $R_{A_1}$ and the one of those in $R_{A_2}$.

\begin{figure}[h]
  	\includegraphics[width=\linewidth]{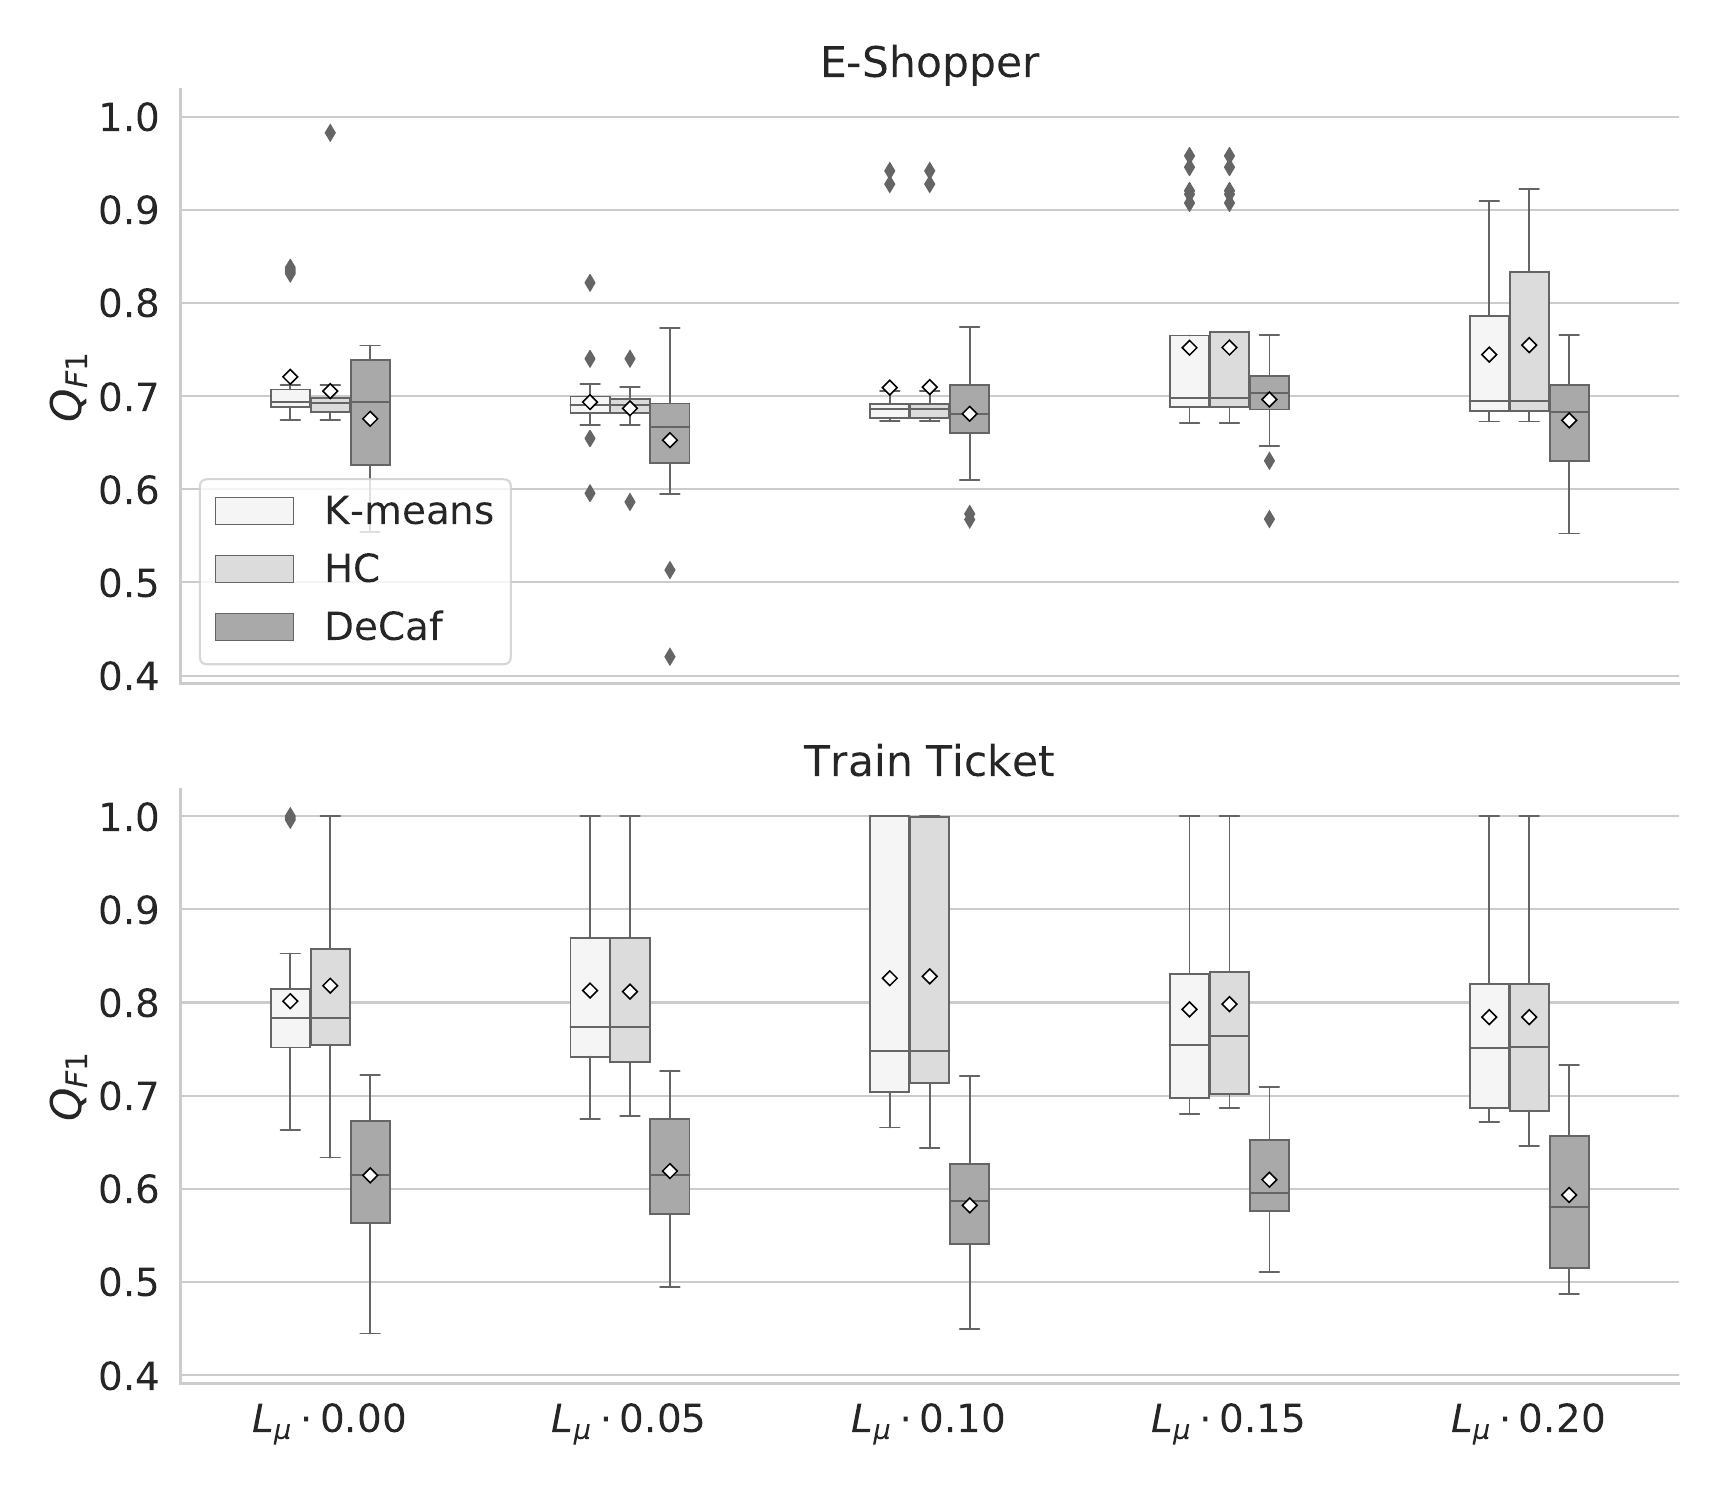}
  	\caption{RQ$_2$. F1-score ($Q_{F1}$) distributions for K-means, HC and DeCaf under the different experimental setups.
  	}
  	\label{fig:rq2_box_others}
\end{figure}

\figref{fig:rq3_box_others} shows distributions for the mean F1-score provided by KrSA, CoTr and DeCaf for each experimental setup defined in \secref{sec:rq3}.
 The x-axis labels report the value of $\widehat{\mathfrak{d}}$,
 i.e. the amount of delay introduced in non-critical RPCs.
 
\begin{figure}[h]
  	\includegraphics[width=\linewidth]{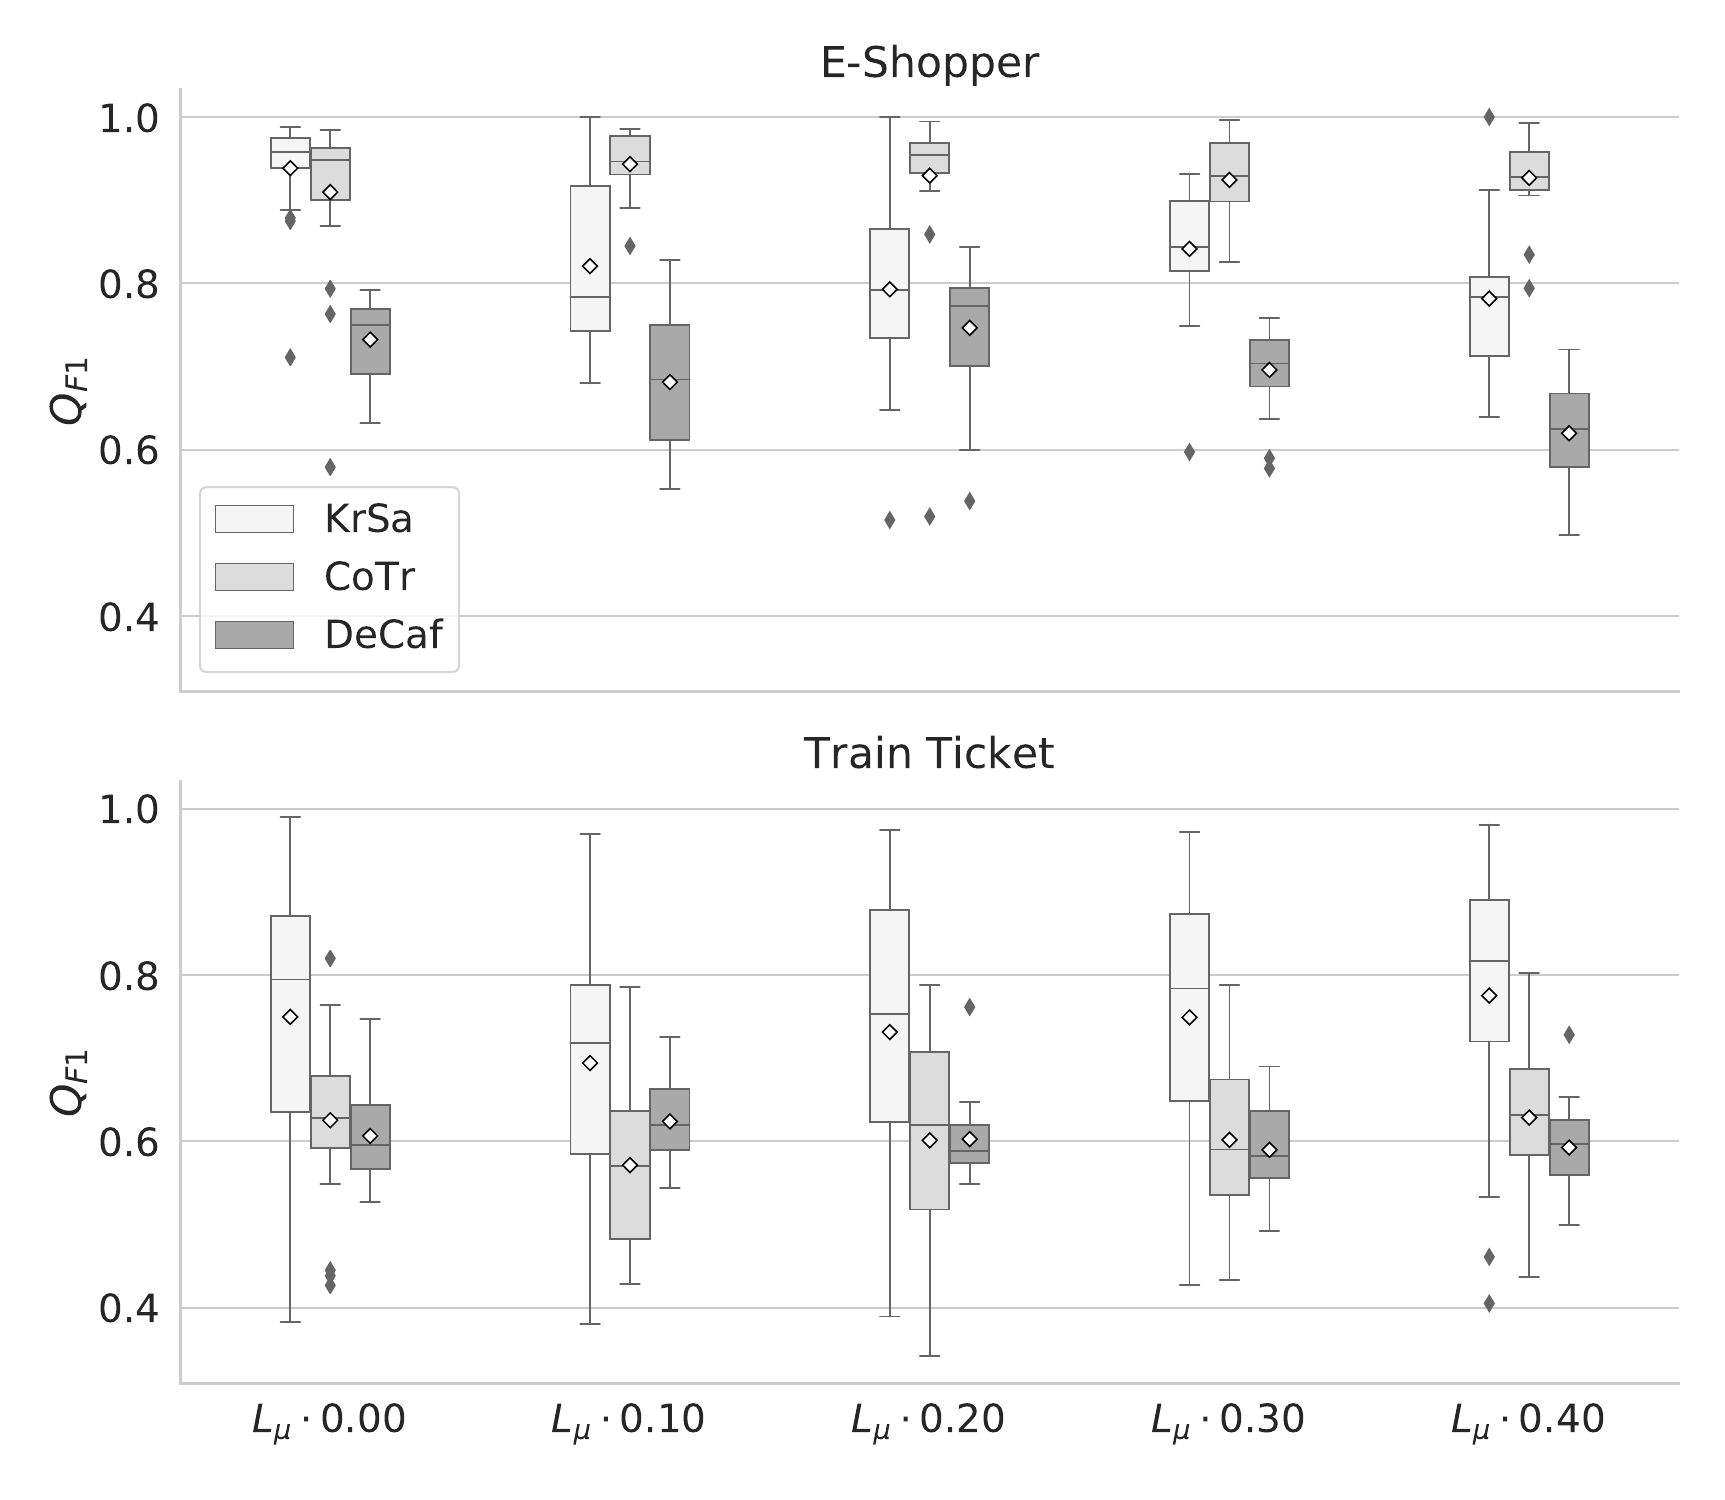}
  	\caption{RQ$_3$. F1-score ($Q_{F1}$) distributions for KrSA, CoTr and DeCaf under the different experimental setups.
  	}
  	\label{fig:rq3_box_others}
\end{figure}
